# Supplementary material for: SMILE: Multimodal Dataset for Understanding Laughter in Video with Language Models
Source: arXiv:2312.09818 source file (2024-05-24)
Supplement: Supplementary file 2 [file supp_AMT_instruction.tex]

\begin{figure}[t]
    \centering
    \includegraphics[width=0.7\textwidth]{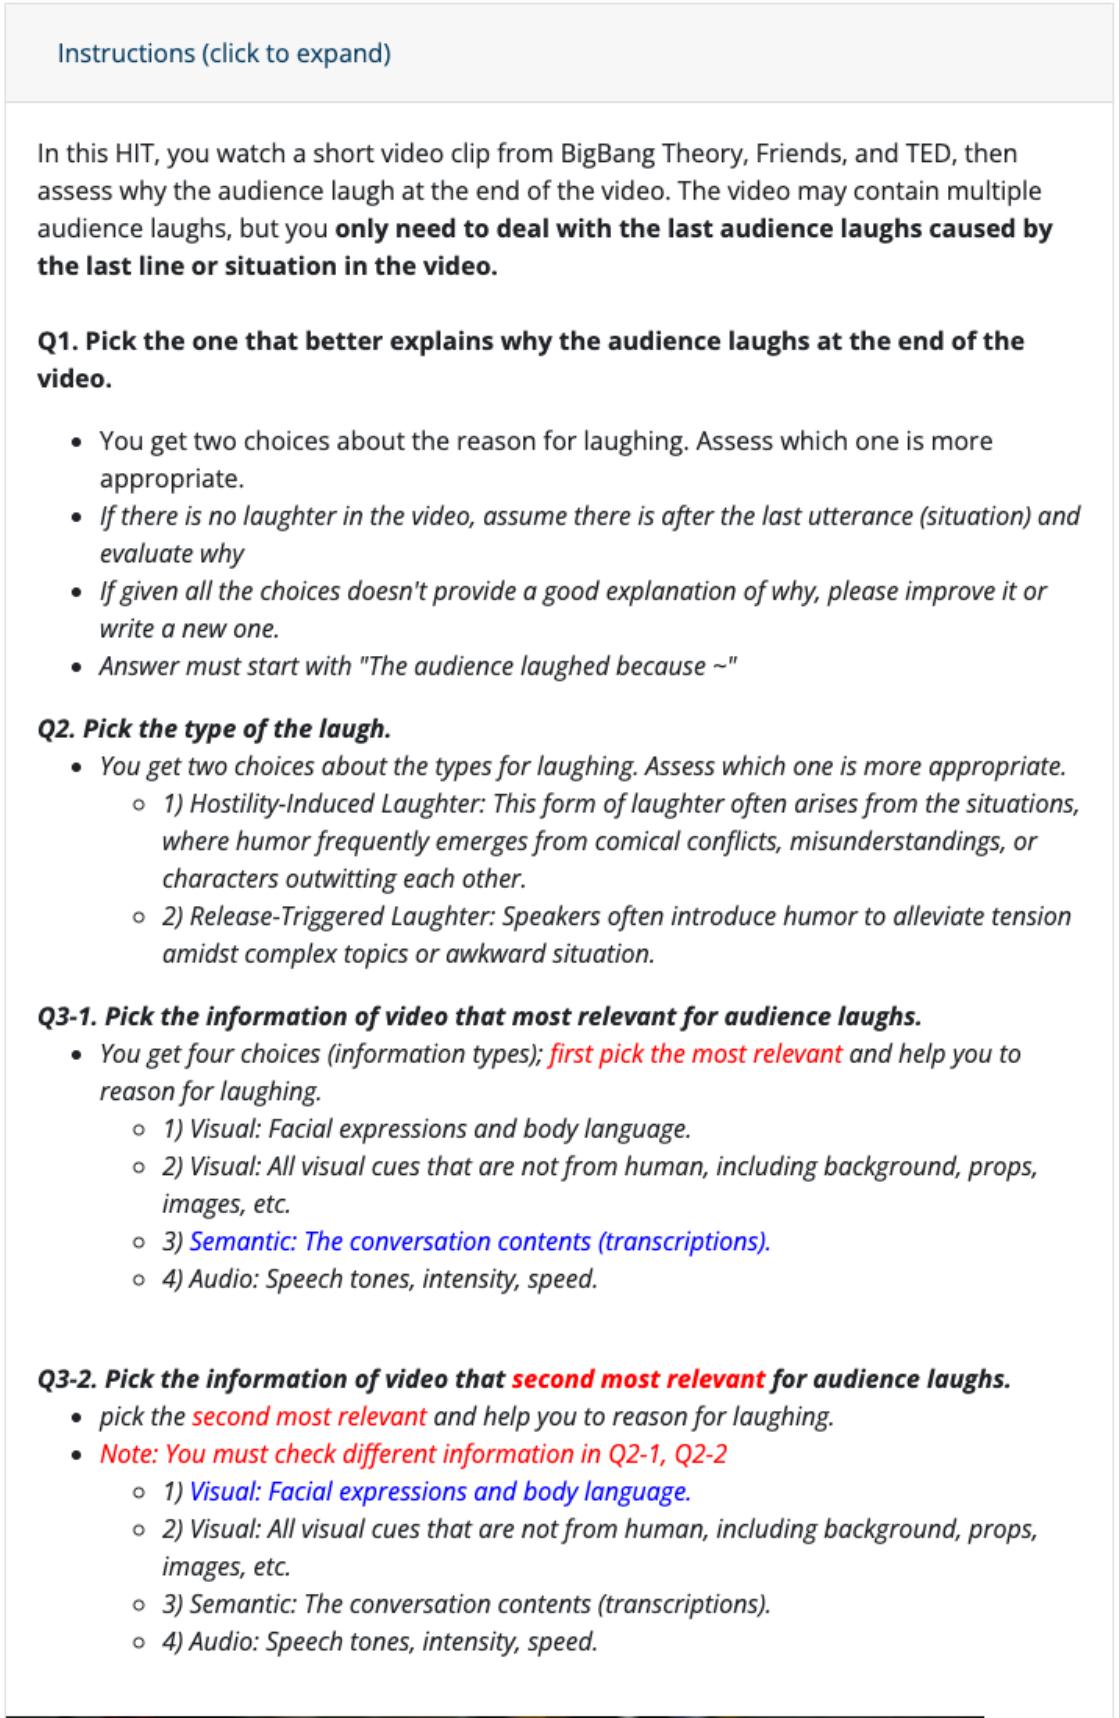}
    \caption{\textbf{Instruction of HITs.} We put the instruction at the top of the interface, describing how the annotators should answer each question.}
    \label{supp_fig:AMT_instruction}
\end{figure}
